# Supplementary material for: T\"oRF: Time-of-Flight Radiance Fields for Dynamic Scene View Synthesis
Source: arXiv:2109.15271 source file (2021-12-06)
Supplement: Supplementary file 1 [file appendix_fig.tex]

\begin{figure}[t]
    \def\imgwidth{0.243\linewidth}
    % \vspace{-\baselineskip}
    \centering
    \begin{tikzpicture}[
		image/.style={inner sep=0pt, outer sep=0pt},
		collabel/.style={above=9pt, anchor=north, inner ysep=0pt, align=center}, % scale=0.8
		rowlabel/.style={left=9pt, rotate=90, anchor=north, inner ysep=0pt, scale=0.8, align=center},
		subcaption/.style={inner xsep=0.75mm, inner ysep=0.75mm, below right},
		arrow/.style={-{Latex[length=2.5mm,width=4mm]}, line width=2mm},
		spy using outlines={rectangle, size=1.5cm, magnification=3, connect spies, ultra thick, every spy on node/.append style={thick}},
		style1/.style={cyan!90!black,thick},
		style2/.style={orange!90!black},
		style3/.style={blue!90!black},
		style4/.style={green!90!black},
	]
	
	\def\padding{2pt}
	% decodearray here is used to remap RGB values in the image to new limits, which we use to brighten the image overall.
    % 	\newcommand{\subfigRGB}[2][0 0 0 0]{\includegraphics[decodearray={0.2 1.2 0.2 1.2 0.2 1.2},width=\imgwidth,trim=#1,clip]{figures/#2.png}}
    % 	\newcommand{\subfigDepth}[2][0 0 0 0]{\includegraphics[width=\imgwidth,trim=#1,clip]{figures/#2.png}}
    %     \newcommand{\subfigDepthTwo}[2][0 0 0 0]{\includegraphics[decodearray={0.0 2.0 0.0 2.0 0.0 2.0},width=\imgwidth,trim=#1,clip]{figures/#2.png}}
    
    \newcommand{\subfigRGB}[2][0 0 0 0]{\includegraphics[decodearray={0.2 1.2 0.2 1.2 0.2 1.2},width=\imgwidth,trim=#1,clip]{figures/#2.png}}
	\newcommand{\subfigDepth}[2][0 0 0 0]{\includegraphics[width=\imgwidth,trim=#1,clip]{figures/#2}}
    \newcommand{\subfigDepthTwo}[2][0 0 0 0]{\includegraphics[width=\imgwidth,trim=#1,clip]{figures/#2}}

	\node [image] (rgb-photocopier) at (0, 0) {\subfigRGB{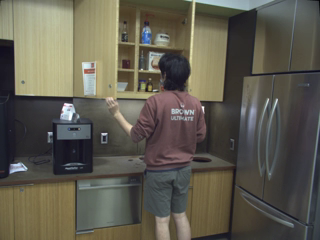}};
	\node [image,right=\padding] (depth-photocopier) at (rgb-photocopier.east) {\subfigDepth{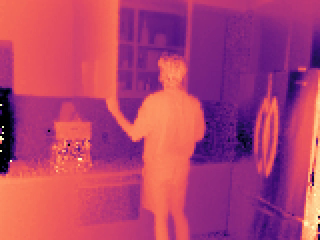}};
    % Right two
	\node [image,right=4pt] (rgb-studybook) at (depth-photocopier.east) {\subfigRGB[20 20 20 10]{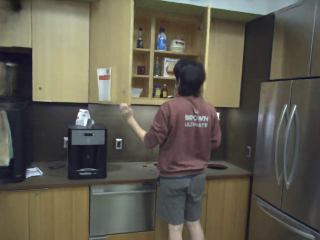}};
	\node [image,right=\padding] (depth-studybook) at (rgb-studybook.east) {\subfigDepthTwo[20 20 20 10]{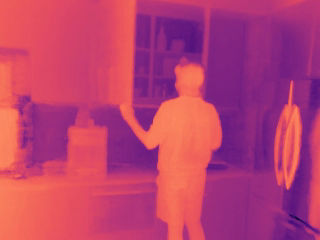}};

    % Top row cut out
	\spy[style3] on ($(rgb-photocopier.center)-(-1.00,-0.1)$) in node (crop-rgb-photocopier) [anchor=south west] at (rgb-photocopier.south west);
	\spy[style3] on ($(depth-photocopier.center)-(-1.00,-0.1)$) in node (crop-depth-photocopier) [anchor=south west] at (depth-photocopier.south west);
	
	% Bottom row cut out
	\spy[style3] on ($(rgb-studybook.center)-(-1.4,0)$) in node (crop-rgb-studybook) [anchor=south west] at (rgb-studybook.south west);
	\spy[style3] on ($(depth-studybook.center)-(-1.4,0)$) in node (crop-depth-studybook) [anchor=south west] at (depth-studybook.south west);

    % Labels
	\node [collabel] at (rgb-photocopier.north)  {\small Color (input)};
	\node [collabel] at (depth-photocopier.north)  {\small Depth (input)};
	\node [collabel] at (rgb-studybook.north)  {\small Color (\torf)};
	\node [collabel] at (depth-studybook.north)  {\small Depth (\torf)};
	
	\end{tikzpicture}
	\caption{The specular reflections from the metallic fridge door results in a C-ToF depth image that does not accurately reflect the true geometry of the door itself.  Instead, the C-ToF camera captures the distance travelled by light reflecting off the fridge door and hitting other objects within the scene. As a result, the reflection of the fridge's door handles appear closer to the camera than the reflection of the cabinets. While not representing the scene's true geometry, we believe that this information guides \torf to more effectively predict the motion of the reflection from novel viewpoints. \label{fig:rawtofvsdepth1}
	}

    \vspace{10pt}
    \def\imgwidth{0.243\linewidth}
    % \vspace{-\baselineskip}
    \centering
    \begin{tikzpicture}[
		image/.style={inner sep=0pt, outer sep=0pt},
		collabel/.style={above=9pt, anchor=north, inner ysep=0pt, align=center}, % scale=0.8
		rowlabel/.style={left=9pt, rotate=90, anchor=north, inner ysep=0pt, scale=0.8, align=center},
		subcaption/.style={inner xsep=0.75mm, inner ysep=0.75mm, below right},
		arrow/.style={-{Latex[length=2.5mm,width=4mm]}, line width=2mm},
		spy using outlines={rectangle, size=1.5cm, magnification=3, connect spies, ultra thick, every spy on node/.append style={thick}},
		style1/.style={cyan!90!black,thick},
		style2/.style={orange!90!black},
		style3/.style={blue!90!black},
		style4/.style={green!90!black},
	]
	
	\def\padding{2pt}
	% decodearray here is used to remap RGB values in the image to new limits, which we use to brighten the image overall.
    % 	\newcommand{\subfigRGB}[2][0 0 0 0]{\includegraphics[decodearray={0.2 1.2 0.2 1.2 0.2 1.2},width=\imgwidth,trim=#1,clip]{figures/#2.png}}
    % 	\newcommand{\subfigDepth}[2][0 0 0 0]{\includegraphics[width=\imgwidth,trim=#1,clip]{figures/#2.png}}
    %     \newcommand{\subfigDepthTwo}[2][0 0 0 0]{\includegraphics[decodearray={0.0 2.0 0.0 2.0 0.0 2.0},width=\imgwidth,trim=#1,clip]{figures/#2.png}}
    
    \newcommand{\subfigRGB}[2][0 0 0 0]{\includegraphics[decodearray={0.2 1.2 0.2 1.2 0.2 1.2},width=\imgwidth,trim=#1,clip]{figures/#2}}
	\newcommand{\subfigDepth}[2][0 0 0 0]{\includegraphics[width=\imgwidth,trim=#1,clip]{figures/#2}}
    \newcommand{\subfigDepthTwo}[2][0 0 0 0]{\includegraphics[width=\imgwidth,trim=#1,clip]{figures/#2}}

	% Left two
    % 	\node [image] (rgb-photocopier) at (0, 0) {\subfigRGB{figure7_rawtofvsdepth/videonerf_photocopier_depthwrap_rgb}};
    % 	\node [image,right=\padding] (depth-photocopier) at (rgb-photocopier.east) {\subfigDepth{figure7_rawtofvsdepth/videonerf_photocopier_depthwrap_depth}};
    \node [image] (rgb-photocopier) at (0, 0) {\subfigRGB{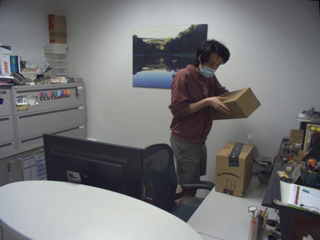}};
	\node [image,right=\padding] (depth-photocopier) at (rgb-photocopier.east) {\subfigDepth{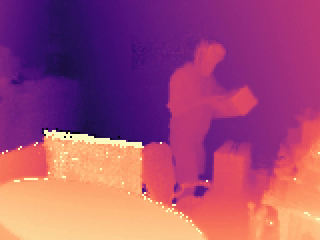}};
    % Right two
	\node [image,right=4pt] (rgb-studybook) at (depth-photocopier.east) {\subfigRGB[20 20 20 10]{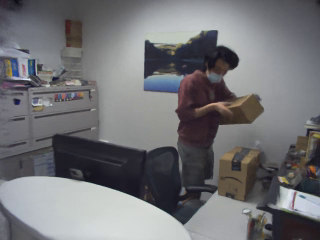}};
	\node [image,right=\padding] (depth-studybook) at (rgb-studybook.east) {\subfigDepthTwo[20 20 20 10]{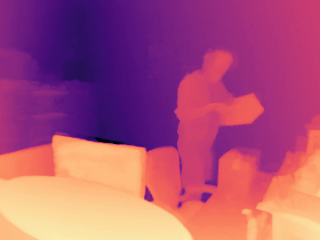}};

    % Top row cut out
	\spy[style3] on ($(rgb-photocopier.center)-(1.1,0.55)$) in node (crop-rgb-photocopier) [anchor=north west] at (rgb-photocopier.north west);
	\spy[style3] on ($(depth-photocopier.center)-(1.1,0.55)$) in node (crop-depth-photocopier) [anchor=north west] at (depth-photocopier.north west);
	
	% Bottom row cut out
	\spy[style3] on ($(rgb-studybook.center)-(1.2,0.6)$) in node (crop-rgb-studybook) [anchor=north west] at (rgb-studybook.north west);
	\spy[style3] on ($(depth-studybook.center)-(1.2,0.6)$) in node (crop-depth-studybook) [anchor=north west] at (depth-studybook.north west);

    % Labels
	\node [collabel] at (rgb-photocopier.north)  {\small Color (input)};
	\node [collabel] at (depth-photocopier.north)  {\small Depth (input)};
	\node [collabel] at (rgb-studybook.north)  {\small Color (\torf)};
	\node [collabel] at (depth-studybook.north)  {\small Depth (\torf)};
	
	\end{tikzpicture}
	\caption{The weak signal reflected back by dark objects (e.g., the computer monitor) results in noisy depth measurements. However, because \torf does not rely on depth explicitly and instead models the raw phasor image, our recovered depth map is a better representation of the scene geometry when compared to the depth extracted from a raw phasor image.\label{fig:rawtofvsdepth2} %\jt{Scene depth scale is off; low priority fix}
	}
\end{figure}
